# Supplementary material for: Taste or Strategy? Nationalistic Bias and Competitor Penalties in Figure Skating Judging
Source: arXiv:2611.13194 source file (2026-11-09)
Supplement: Supplementary file 1 [file notes_appendix_D.tex]

% the Appendix D notes of the main tables, one macro each (py-main/p1_tex.py from s-manual/paper1.spec's
% `notes` entries): \AppDNoteTable<N>, N the table's number in words; then the footnotes of the tables
% that have one (`footnote` entries), one macro each under the name the spec gives
\newcommand{\AppDNoteTableThree}{\paragraph{Table 3.} Standard errors are two-way clustered by competition and skater (Cameron, Gelbach and Miller 2011). Clustering by competition and the skater's federation instead gives standard errors 0.86--1.85 times those shown and changes no star. The two-way cluster jackknife of MacKinnon, Nielsen and Webb (2026) on competition and skater gives standard errors 1.01--1.06 times those shown and changes the stars of Rival in column (3) from the 1\% level to the 5\% level.}
\newcommand{\AppDNoteTableFour}{\paragraph{Table 4.} Standard errors are two-way clustered by competition and skater (Cameron, Gelbach and Miller 2011). Clustering by competition and the skater's federation instead gives standard errors 0.83--1.84 times those shown and changes the stars of Rival starting later, in contention in column (1) from the 1\% level to the 5\% level; Rival starting later, out of contention in column (2) from the 5\% level to no star; Rival starting earlier in column (4) from the 10\% level to the 5\% level. The two-way cluster jackknife of MacKinnon, Nielsen and Webb (2026) on competition and skater gives standard errors 1.01--1.07 times those shown and changes no star.}
\newcommand{\AppDNoteTableFive}{\paragraph{Table 5.} Standard errors are two-way clustered by competition and skater (Cameron, Gelbach and Miller 2011). Clustering by competition and the skater's federation instead gives standard errors 0.60--1.66 times those shown and changes the stars of Rival in column (1) from the 1\% level to the 10\% level; Other-panel compatriot in column (1) from the 5\% level to the 10\% level; Rival in column (7) from no star to the 10\% level; Other-panel compatriot in column (9) from the 10\% level to the 5\% level. The two-way cluster jackknife of MacKinnon, Nielsen and Webb (2026) on competition and skater gives standard errors 1.01--1.48 times those shown and changes the stars of Rival in column (1) from the 1\% level to the 5\% level; Compatriot Technical Controller in column (1) from the 5\% level to the 10\% level; Compatriot Technical Controller in column (4) from the 5\% level to the 10\% level; Compatriot Technical Controller in column (7) from the 5\% level to the 10\% level.}
\newcommand{\AppDNoteTableSix}{\paragraph{Table 6.} Standard errors are two-way clustered by competition and skater (Cameron, Gelbach and Miller 2011). Clustering by competition and the skater's federation instead gives standard errors 0.73--1.60 times those shown for the slope cells of Appendix Table~A.18: of the 24 (19 starred), 4 change stars (2 gaining, 2 losing). The two-way cluster jackknife of MacKinnon, Nielsen and Webb (2026) on competition and skater gives standard errors 1.14--1.36 times those shown for the slope cells of Appendix Table~A.18: of the 24 (19 starred), 9 change stars (0 gaining, 9 losing).}
\newcommand{\AppDNoteTableSeven}{\paragraph{Table 7.} Standard errors are two-way clustered by competition and skater (Cameron, Gelbach and Miller 2011). Clustering by competition and the skater's federation instead gives standard errors 0.45--1.51 times those shown for the interaction cells of Appendix Table~A.19: of the 36 (7 starred), 3 change stars (1 gaining, 2 losing). The two-way cluster jackknife of MacKinnon, Nielsen and Webb (2026) on competition and skater gives standard errors 1.12--1.69 times those shown for the interaction cells of Appendix Table~A.19: of the 36 (7 starred), 6 change stars (0 gaining, 6 losing).}
\newcommand{\AppDNoteTableEight}{\paragraph{Table 8.} Standard errors are two-way clustered by competition and skater (Cameron, Gelbach and Miller 2011). Clustering by competition and the skater's federation instead gives standard errors 0.61--1.91 times those shown for the interaction cells of Appendix Table~A.20: of the 36 (5 starred), 3 change stars (2 gaining, 1 losing). The two-way cluster jackknife of MacKinnon, Nielsen and Webb (2026) on competition and skater gives standard errors 1.15--1.66 times those shown for the interaction cells of Appendix Table~A.20: of the 36 (5 starred), 4 change stars (0 gaining, 4 losing).}
\newcommand{\AppDNoteTableNine}{\paragraph{Table 9.} Standard errors are two-way clustered by competition and skater (Cameron, Gelbach and Miller 2011). Clustering by competition and the skater's federation instead gives standard errors 0.55--1.53 times those shown for the interaction cells of Appendix Table~A.21: of the 36 (9 starred), 4 change stars (1 gaining, 3 losing). The two-way cluster jackknife of MacKinnon, Nielsen and Webb (2026) on competition and skater gives standard errors 1.16--1.54 times those shown for the interaction cells of Appendix Table~A.21: of the 36 (9 starred), 9 change stars (0 gaining, 9 losing).}
\newcommand{\AppDFootnoteTableSix}{Each slope is the one in Table 6, with the stars of that table's standard error: two-way cluster-robust by competition and skater (Cameron, Gelbach and Miller 2011), its $p$-value against $t$ with $G-1$ degrees of freedom. In parentheses: its standard error two-way cluster-robust by competition and the skater's federation, with the stars of its $p$-value against $t$ with $\min(G,F)-1$ degrees of freedom. A two-way cluster-robust variance is the sum of the variances clustered by each of the two dimensions less the variance clustered by their intersection, each with the factor $c/(c-1)$ of its $c$ clusters. In brackets: the two-way cluster jackknife standard error of MacKinnon, Nielsen and Webb (2026) by competition and skater, the square root of the largest of $V_G+V_H-V_I$, $V_G$ and $V_H$, where $V_G$, $V_H$ and $V_I$ are the jackknife variances $\frac{J-1}{J}\sum_{j}(\hat\beta_{(j)}-\hat\beta)^2$ of the estimates that leave out one of the $J$ competitions, skaters or competition-skater pairs at a time (with the coefficient of a cell dummy left without rows set to zero), with the stars of its $p$-value against $t$ with $\min(G,H)-1$ degrees of freedom. $G$, $H$ and $F$ are the column's competitions, skaters and skater federations. $^{*}$ $p<0.10$, $^{**}$ $p<0.05$, $^{***}$ $p<0.01$.}
\newcommand{\AppDFootnoteTableSeven}{Each interaction is the one in Table 7, with the stars of that table's standard error: two-way cluster-robust by competition and skater (Cameron, Gelbach and Miller 2011), its $p$-value against $t$ with $G-1$ degrees of freedom. In parentheses: its standard error two-way cluster-robust by competition and the skater's federation, with the stars of its $p$-value against $t$ with $\min(G,F)-1$ degrees of freedom. A two-way cluster-robust variance is the sum of the variances clustered by each of the two dimensions less the variance clustered by their intersection, each with the factor $c/(c-1)$ of its $c$ clusters. In brackets: the two-way cluster jackknife standard error of MacKinnon, Nielsen and Webb (2026) by competition and skater, the square root of the largest of $V_G+V_H-V_I$, $V_G$ and $V_H$, where $V_G$, $V_H$ and $V_I$ are the jackknife variances $\frac{J-1}{J}\sum_{j}(\hat\beta_{(j)}-\hat\beta)^2$ of the estimates that leave out one of the $J$ competitions, skaters or competition-skater pairs at a time (with the coefficient of a cell dummy left without rows set to zero), with the stars of its $p$-value against $t$ with $\min(G,H)-1$ degrees of freedom. The second step is corrected for the sampling error of the first step's trained premia, and each of the three variances adds the first step's term (as in Table 7); the jackknife estimates the corrected second step without each cluster in turn, the cluster's share of the correction leaving with its rows. $G$, $H$ and $F$ are the column's competitions, skaters and skater federations. $^{*}$ $p<0.10$, $^{**}$ $p<0.05$, $^{***}$ $p<0.01$.}
\newcommand{\AppDFootnoteTableEight}{Each interaction is the one in Table 8, with the stars of that table's standard error: two-way cluster-robust by competition and skater (Cameron, Gelbach and Miller 2011), its $p$-value against $t$ with $G-1$ degrees of freedom. In parentheses: its standard error two-way cluster-robust by competition and the skater's federation, with the stars of its $p$-value against $t$ with $\min(G,F)-1$ degrees of freedom. A two-way cluster-robust variance is the sum of the variances clustered by each of the two dimensions less the variance clustered by their intersection, each with the factor $c/(c-1)$ of its $c$ clusters. In brackets: the two-way cluster jackknife standard error of MacKinnon, Nielsen and Webb (2026) by competition and skater, the square root of the largest of $V_G+V_H-V_I$, $V_G$ and $V_H$, where $V_G$, $V_H$ and $V_I$ are the jackknife variances $\frac{J-1}{J}\sum_{j}(\hat\beta_{(j)}-\hat\beta)^2$ of the estimates that leave out one of the $J$ competitions, skaters or competition-skater pairs at a time (with the coefficient of a cell dummy left without rows set to zero), with the stars of its $p$-value against $t$ with $\min(G,H)-1$ degrees of freedom. The second step is corrected for the sampling error of the first step's trained premia, and each of the three variances adds the first step's term (as in Table 8); the jackknife estimates the corrected second step without each cluster in turn, the cluster's share of the correction leaving with its rows. $G$, $H$ and $F$ are the column's competitions, skaters and skater federations. $^{*}$ $p<0.10$, $^{**}$ $p<0.05$, $^{***}$ $p<0.01$.}
\newcommand{\AppDFootnoteTableNine}{Each interaction is the one in Table 9, with the stars of that table's standard error: two-way cluster-robust by competition and skater (Cameron, Gelbach and Miller 2011), its $p$-value against $t$ with $G-1$ degrees of freedom. In parentheses: its standard error two-way cluster-robust by competition and the skater's federation, with the stars of its $p$-value against $t$ with $\min(G,F)-1$ degrees of freedom. A two-way cluster-robust variance is the sum of the variances clustered by each of the two dimensions less the variance clustered by their intersection, each with the factor $c/(c-1)$ of its $c$ clusters. In brackets: the two-way cluster jackknife standard error of MacKinnon, Nielsen and Webb (2026) by competition and skater, the square root of the largest of $V_G+V_H-V_I$, $V_G$ and $V_H$, where $V_G$, $V_H$ and $V_I$ are the jackknife variances $\frac{J-1}{J}\sum_{j}(\hat\beta_{(j)}-\hat\beta)^2$ of the estimates that leave out one of the $J$ competitions, skaters or competition-skater pairs at a time (with the coefficient of a cell dummy left without rows set to zero), with the stars of its $p$-value against $t$ with $\min(G,H)-1$ degrees of freedom. Every trained premium is set to 1 (Table 9): no first step enters. $G$, $H$ and $F$ are the column's competitions, skaters and skater federations. $^{*}$ $p<0.10$, $^{**}$ $p<0.05$, $^{***}$ $p<0.01$.}
